# Supplementary material for: Deep learning enabled design of complex transmission matrices for universal optical components
Source: arXiv:2009.11810 ancillary file (2020-12-08)
Supplement: Supplementary file 1 [file DinsdaleMMI2020_SI.pdf]

# Supporting information for "Deep learning enabled design of complex transmission matrices for universal optical components"

Nicholas J. Dinsdale,[1,2] Peter R. Wiecha,[2,3,*] Matthew Delaney,[1,2] Jamie Reynolds,[1] Martin Ebert,[1] Ioannis Zeimpekis,[1] David J. Thomson,[1] Graham T. Reed,[1] Philippe Lalanne,[4] Kevin Vynck,[4] and Otto L. Muskens[2,†]

[1]*Optoelectronics Research Centre, University of Southampton, Southampton, UK*
[2]*Physics and Astronomy, Faculty of Engineering and Physical Sciences, University of Southampton, SO17 1BJ Southampton, UK*
[3]*LAAS, Université de Toulouse, CNRS, Toulouse, France*
[4]*LP2N, CNRS - Institut dOptique Graduate School - Univ. Bordeaux, F-33400 Talence, France*

## I. SUPPORTING INFORMATION

### A. Data-generation

For the ANN's ability to generalize well, we need to generate random transmission matrix targets for both the initial training dataset, iterative training sample generation, as well as for the statistical testing of the ANN performance. In this procedure, we first define a target device total transmittance, taking into account that our platform usually produces losses in the order of $10-30\%$.

*a. Initial training data optimization* For the optimization of patterns in the initial training dataset ("step 0"), the total target transmittance is fixed to 100% and the splitting ratio between output ports is randomized. The deviation of the MMI to the target transmission matrix is described the following fitness function, which is then maximized during the iterative pattern-generation:

$$f = 1 - \left[ \sum_{m=1}^{M} \sum_{n=1}^{N} \left( T_{m,n}^{\text{tar}} - T_{m,n} \right)^2 \right]^{0.5} . \quad \text{(S1)}$$

Here $T_{m,n}^{\text{tar}}$ and $T_{m,n}$ are the target, respectively modelled total transmittance for the corresponding coupling between the $m^{\text{th}}$ input and $n^{\text{th}}$ output ports.

Figure S1a illustrates an example of pattern generation for the iterative optimization of coupling towards a single output of a $1 \times 2$ MMI using the a-FMM solver. The colored circles correspond to the perturbation patterns, and their FDTD simulated electric field distributions and intensity profiles shown in Figure S1b.

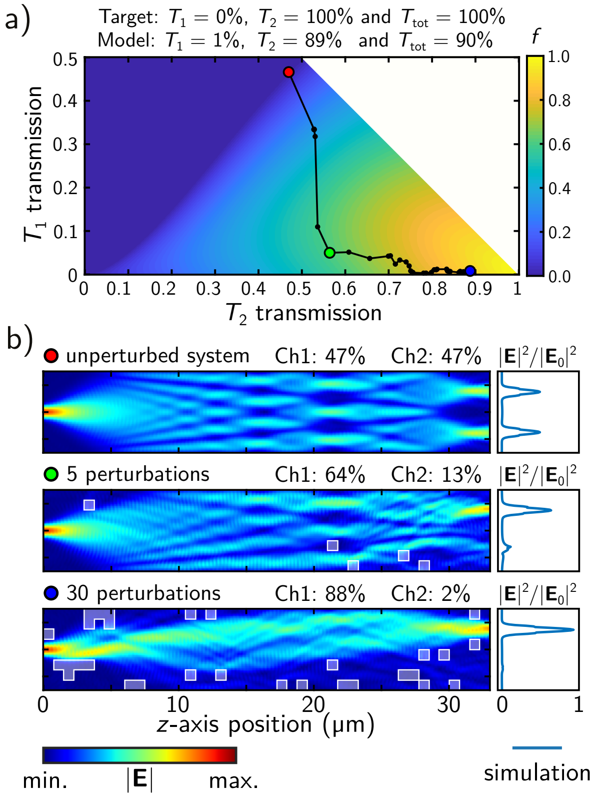


Figure S1. (a) optimisation of a perturbation pattern for a specific target transmission state, here Ch.1–0% and Ch.2–100%. (b) iteratively designed randomized MMI patterns with corresponding FDTD simulated $|\mathbf{E}|$ field distributions (colormaps) and intensity profiles across the output waveguides (blue lines in right subplots). Coloured circles in (a) correspond to the accordingly labeled simulated patterns in (b).

### B. ANN details and hyperparameters

Typical convergence plots of loss vs. training epoch are shown in figure S2a and S2b for the forward, respectively generator networks.

### C. Binary pattern threshold determination

Deep learning network training is an optimization process relying on the gradients of the ANN output with respect to the internal network parameters. Hence, the output of an ANN is necessarily continous, whereas our MMI designs are binary. Therefore we need to apply a threshold value to transform the greyscale ANN designs into binary perturbation patterns. As described in the main text, the best threshold can be obtained using the forward network for testing of the MMI performance. Practically, various levels of perturbations could be introduced experimentally via different etch heights, however, this would require additional fabrication steps. With regards to the weaker optical perturbations considered, some intensity

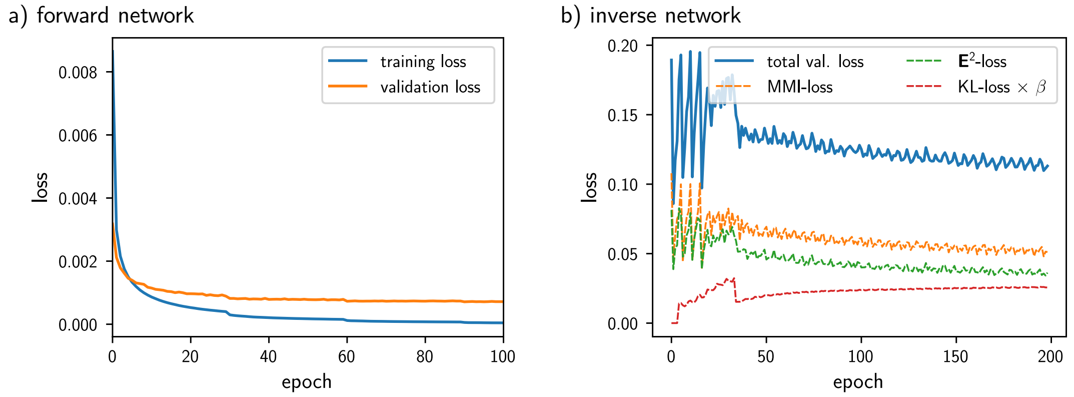


Figure S2. Example of loss convergence during (a) forward and (b) generator network training.

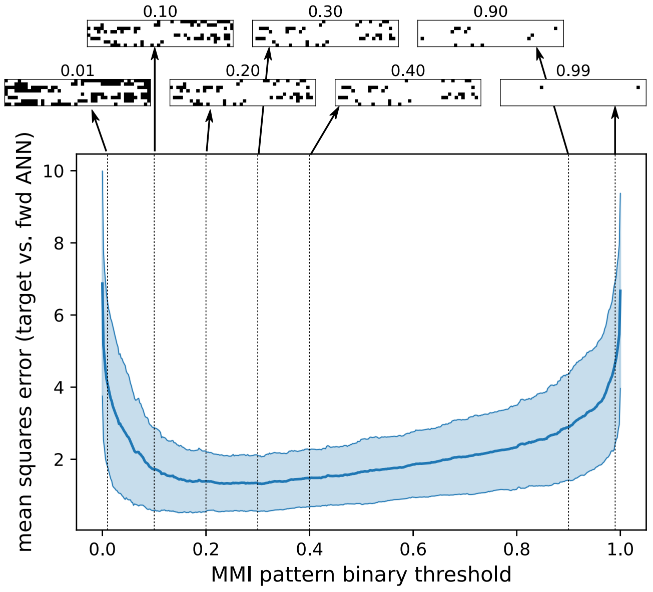


Figure S3. Mean squares error between design target and forward network predicted MMI intensity profile averaged for 150 inverse designed test MMIs as function of the threshold value. Thick blue line is the mean of the test-set, the shaded area corresponds to the standard deviation. A selected MMI is shown at the top, converted from grey-scale to binary using different threshold values (indicated with the label at the top).

modulation could be applied to each projected pump spot to achieve a similar control over the refractive index change. In figure S3 we show the mean square error between target and ANN-designed MMI as function of the threshold value. The blue line is the average of 150 test cases, the shaded area corresponds to the standard deviation. At the top, perturbation patterns of a selected example are shown for several threshold values to illustrate the impact on the MMI. As can be seen, between threshold values around 0.2 and 0.4, the design error has a plateau-like minimum and the pattern is almost unchanged. If inverse-design speed should need to be further increased, the threshold could be fixed to a value in the center of this plateau, reducing the inverse design time from around 50 ms to the order of 1 ms.

## D. ANN validation statistics and additional inverse design examples

Figures S4a and S4b show the average absolute peak intensity error of the forward and generator ANNs, respectively, for each of the six generations of the etched $1 \times 2$ MMI iterative training scheme. The errors are calculated by comparing predicted and simulated outputs of the validation dataset, which remain unseen by the networks during training, and are plotted against the number of perturbations contained by a pattern. The mean total error for any number of perturbations is given by the dashed line and subsequent iterations are indicated by the darker colour of a particular line. The initial generation of the forward network shows very poor prediction with around a 5% average error that rapidly deteriorates with increasing number of perturbations. Later iterations have significantly less error (around 1% for iteration 5) and a much flatter response to number of perturbations. The generator networks show a similar improvement with increasing iterations, however, the error overall is slightly higher as the generator itself also utilises the forward predictor network.

Similarly, the average absolute peak intensity error of the forward and generator ANNs for each of the six generations of the $3 \times 3$ MMI iterative training scheme are shown by figures S5a and S5b, respectively. Once again, later iterations are indicated by darker line colours and the average error is compared to the number of perturbations contained by a pattern, but now the error is evaluated for each of the three input channels. Unlike the etched $1 \times 2$ MMI case, the forward network for the $3 \times 3$ device continues to display a degradation of prediction performance with increasing number of perturbations, even for later iterations. This is attributed to the increased complexity of the system and higher average number of perturbations contained in a pattern. The generator network, however, shows a much flatter response after the first 8 accepted perturbations. Both the forward and generator ANNs show improved performance with later iteration with average

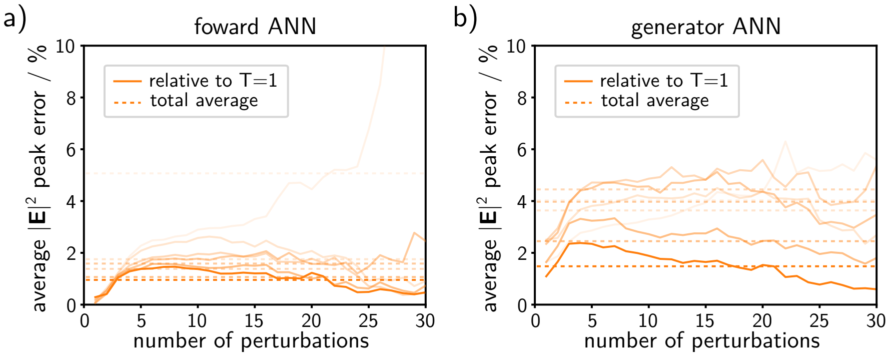


Figure S4. $1\times2$ MMI (a) forward and (b) generator ANN average absolute output peak intensity error calculated from the validation dataset for each of the iterations. Increasing iterations are indicated by line colour transitioning from light to dark and dashed line shows the total average error.

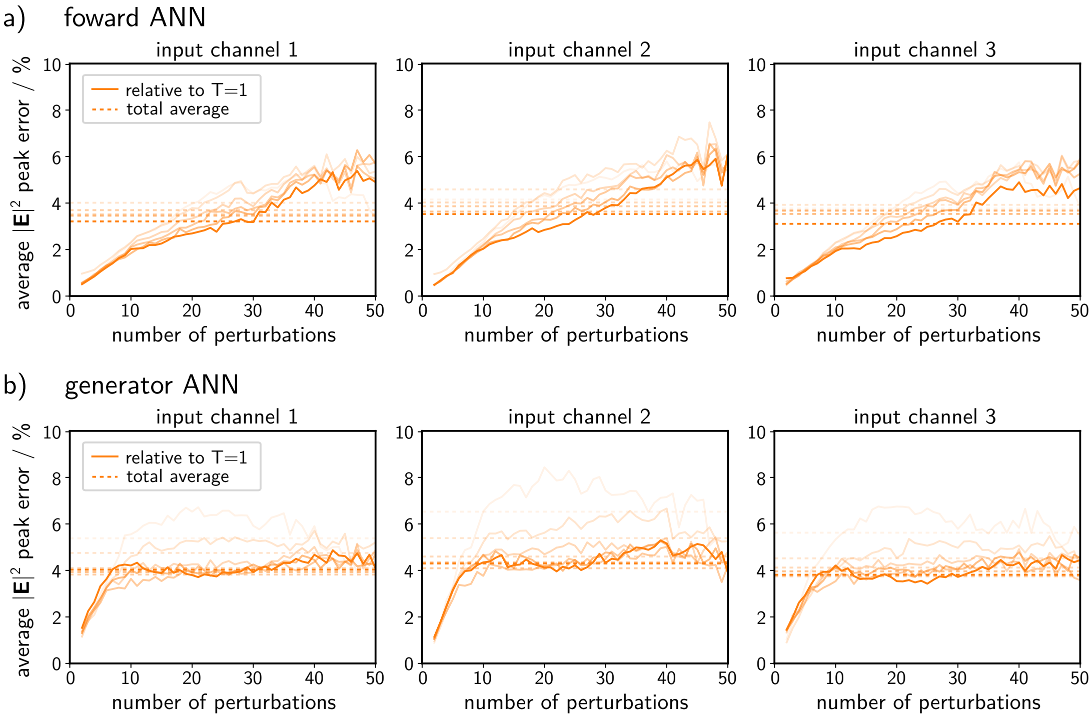


Figure S5. $3\times3$ MMI (a) forward and (b) generator ANN average absolute output peak intensity error calculated from the validation dataset for each of the iterations and input channels. Increasing iterations are indicated by line colour transitioning from light to dark and dashed line shows the total average error.

errors of less than 4%.

Examples of inverse designed etched $1\times2$ MMI patterns are shown in figure S6 for different transmittance splitting ratios, smoothly switching the output from channel 1 (top left) to 2 (top right), with a 90% total transmittance target. Patterns were generated by the final iteration of the networks and their corresponding electric field distributions and output intensity profiles were calculated by FDTD simulation. The 45%:45% target case is not shown as it corresponds basically to an empty MMI, the target being very close to the splitting performance of the unperturbed device of 47%:47%. In all cases the agreement between target, prediction and simulation is excellent, as one would expect from performance statistics shown in figure S4. Since the method is data-driven, the network does not necessarily find symmetric patterns for vertically flipped design targets. Note that the right-hand side column cases are identical to the results shown in main text figure 2f and repeated here for ease of comparison.

The remaining two perturbation patterns, and their corresponding electric field distributions, for the complete set of input-output permutations of the $3\times3$ MMI inverse design examples (figure 4 of the main text) are shown in figure S7a. These have transmittance targets that bare symmetry to previous shown examples, corresponding to flipping the device about the long axis. The complete set of transmission matrices for the port permutation case are then shown in figure S7b,

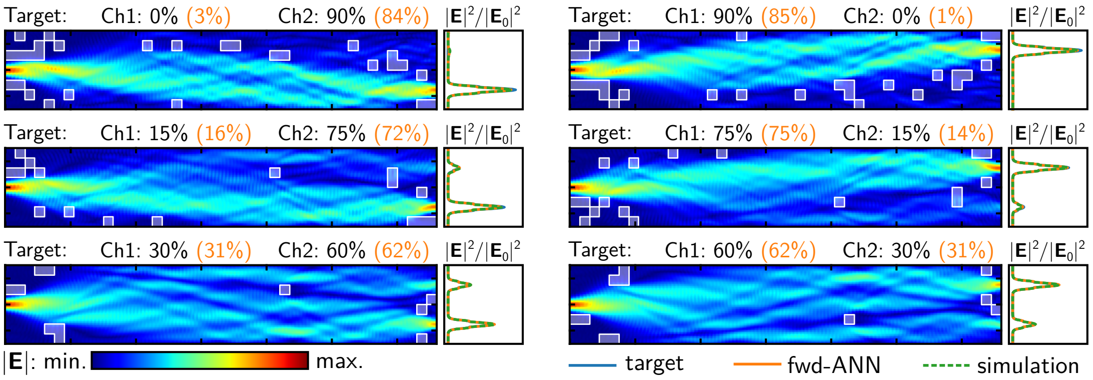


Figure S6. Examples of inverse designed $1 \times 2$ MMI perturbation patterns with a 90% total transmittance target. Patterns are generated from the iteration 5 network and their corresponding electric field distributions and output intensity profiles were calculated by FDTD simulation. The target transmittance values for each output port are listed above the electric field distribution (simulated transmission is given in orange), for different splitting ratios switching the output between channel 1 and 2. To the right of the electric field distributions are the intensity profiles along the output waveguides for design target (solid blue lines), forward-ANN (solid orange lines) and FDTD simulation (dashed green lines).

as well as for the additional cases where one port coupling is unitary and the other two are split 50:50 between the remaining outputs. The total transmittance target for each input port was limited to 80% in all cases. The general agreement is very good as shown by the transmission error matrices, however, some specific port couplings have transmittance errors as high as 20%. Note again that the network does not find symmetric patterns for vertically flipped design targets, also the performance of symmetric cases is not identical. This is a result of the model being data-driven.

### E. Further phase-aware inverse design examples

In figure S8 we show additional examples for phase-aware inverse design. The color hue and brightness represent the complex phase and amplitude at the output of the device normalized to the input amplitude, as indicated by the color-legend in the figure centre. Subfigures S8a-d represent fixed intensity patterns, for each of which the phase is rotated through a $2\pi$ cycle. Fig. S8d shows the same intensity pattern as main text figure 6, with an additional relative phase of $\pi/6$ between the individual output channels.

### F. Compare inverse design to training data

In order to assess whether the inverse ANN developed a general understanding of the inverse design problem or if it only acts as a kind of lookup table for the training data, we compared each inverse design pattern of the test-set to the full set of training samples. To quantify the “originality” of an inverse design, we search the training set for the most similar sample, hence the pattern with the least number of different perturbation positions in comparison to the ANN design. In table S1 we show the average number of non-identical perturbation positions and its standard deviation for the generator network trained on either the initial dataset only, or on the

Table S1. Average number of mismatching perturbations between the inverse designs and the most similar MMI pattern in the training set. The table compares the two different MMI-types and ANN models, trained either only on the initial dataset or via the iterative training. The error corresponds to the standard deviation. The second value is the average number of perturbations of the inverse designed MMIs patterns

| MMI type / dataset | most similar training sample avg. mismatch count / total pert. count |
|---|---|
| $1 \times 2$ / initial data only | $10.1 \pm 10.2$ / $19.1 \pm 15.0$ |
| $1 \times 2$ / iterative training | $1.9 \pm 1.5$ / $16.1 \pm 5.1$ |
| $3 \times 3$ / initial data only | $21.4 \pm 12.5$ / $45.6 \pm 20.9$ |
| $3 \times 3$ / iterative training | $17.1 \pm 12.2$ / $36.0 \pm 13.6$ |

dataset after 5 full training iterations. While after the iterative training, the $1 \times 2$ generator seems to become some kind of lookup table for the best matching training-set sample ($< 2$ different perturbation positions), in the $3 \times 3$ case, the network does generally not reproduce a pattern from the training set, but produces original MMI designs.

### G. MMI experimental insertion loss

In the perturbed device we experimentally observe a slightly increased excess loss (bare MMI: $-0.7242$ dB versus optimized pattern etched MMI: $-0.9151$ dB). The values are obtained by comparison to a measurement on a straight waveguide under otherwise identical conditions.

### H. MMI losses - 2D vs. 3D simulations

In order to assess the fidelity of the 2D FDTD simulations, we perform a comparison with 3D FDTD simulations. 3D

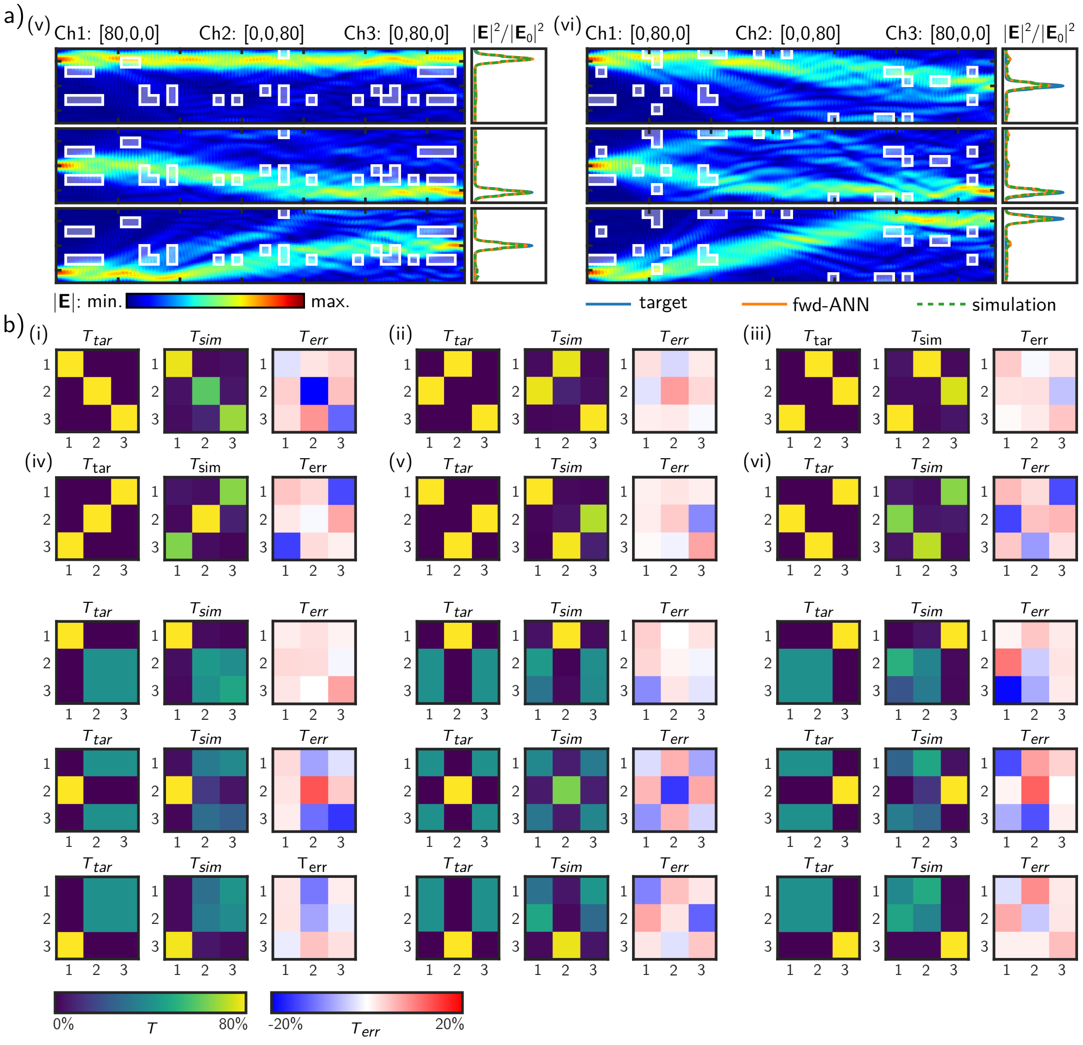


Figure S7. (a) FDTD simulated electric field distributions and output waveguide intensity profiles of the remaining two $3 \times 3$ MMI inverse design examples (v-vi) from figure 4 of the main text. Patterns are generated from the iteration 5 network. Transmission matrices for all six input-output permutation cases (roman numerals correspond to part (a) and figure 4 of the main text), as well as for the additional cases where one port coupling is unitary and the other two are split 50:50 between the remaining outputs. The total transmittance target is set to 80%.

simulations take significantly more time (2D: tens of seconds, 3D: order of an hour), therefore creating a training set with real 3D simulations would require important computational capacities. As illustrated in figure S10 by typical optimized $1 \times 2$ MMI patterns for (a) etched and (b) optical perturbations, we find that the 2D approximation is very good, with deviations of not more than a few percent. The differences can be explained by out-of-plane scattering, which is not described by the 2D simulations (see below). The good agreement, in particular in the case of optical perturbations, justifies the use of the 2D effective index approximation for the neural network training data generation.

## I. MMI out of plane scattering - 3D simulations

The main reason for deviations between the 2D and 3D models is out-of-plane scattering. We therefore perform 3D FDTD simulations of the scattering losses in a waveguide model with a single perturbation (see table S2. This configuration illustrates the worst-case scenario, where the entire light flux is forced to pass through the perturbation. Accordingly, the scattering losses are notable. In particular in the case of a fully etched perturbation the total loss sums up to around 30%. Shallow etching helps to reduce these losses quite significantly, this corresponds to the fabrication conditions of our rib waveguide MMI. Finally, optical perturbations are found to induce very little scattering.

In addition to the single-perturbation waveguide, we simulate out-of-plane scattering losses in a patterned MMI (see table S3). In contrast to the lossless transmission through the

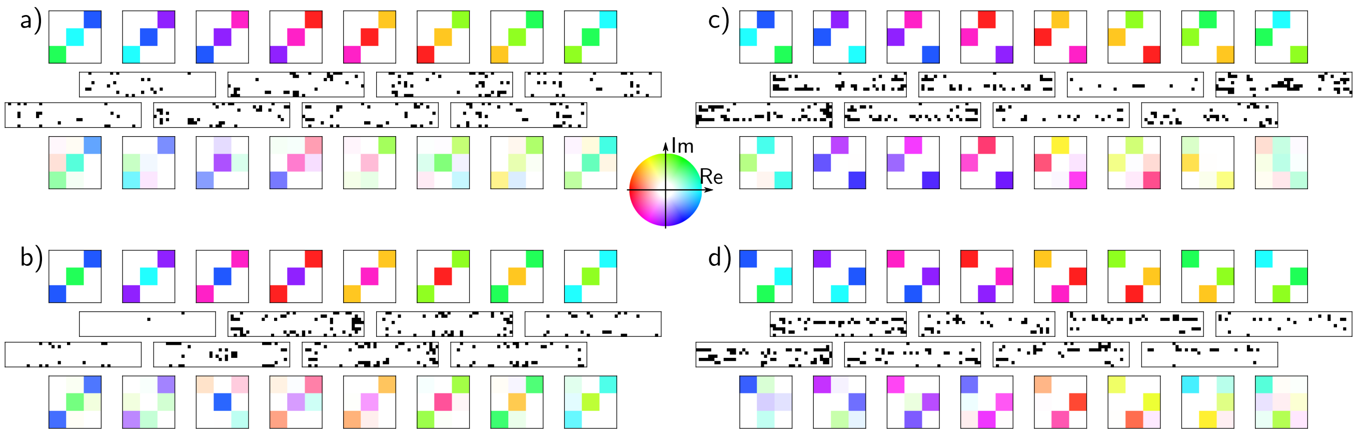


Figure S8. More examples of phase-aware inverse design. a)-d) show a fixed intensity and relative phase layout, for which the phase is rotated through a $2\pi$ cycle. Top rows show the complex field target, the center rows the ANN-designed MMI, and the bottom rows the FDTD simulated complex transmission matrix. d) shows the same case as in main text figure 6, but here with an additional relative phase of $\pi/6$ between each non-zero output channel.

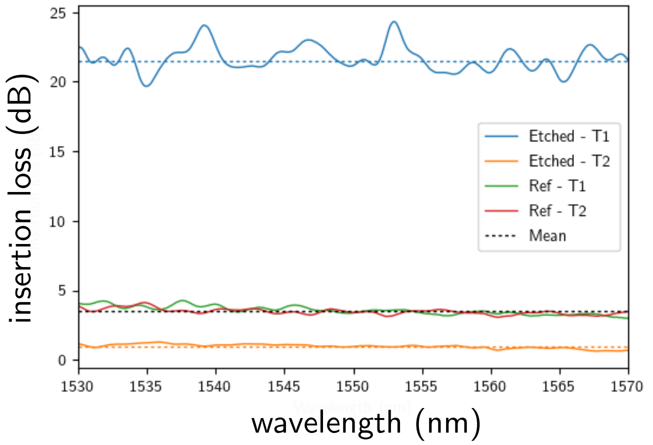


Figure S9. Measured losses of the optimised, etched $1 \times 2$ device (c.f. main text figure 2) for transmission to the upper and lower output channels (T1: blue, respectively T2: orange). For comparison, the insertion loss of an unperturbed bare MMI is shown (green and red lines).

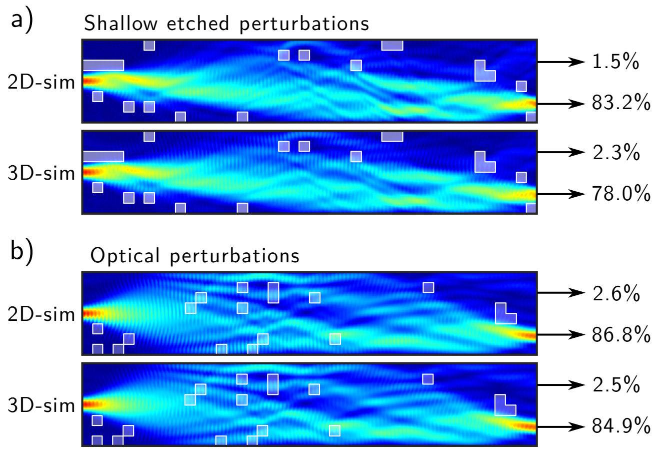


Figure S10. Comparison of 2D and 3D FDTD simulations for $1 \times 2$ MMIs with a) shallow etched perturbations (as in our experimental test) and b) optical perturbations. In both cases, the top image corresponds to the 2D effective index simulations, the bottom image to the full 3D simulation.

bare waveguide, already the unperturbed MMI suffers from weak losses in the order of one percent, which is a result of scattering at the output facet. By the inverse design process a pattern is created which minimizes light-flux through the perturbations. This actually reduces the scattering losses in comparison with the aforementioned single-perturbation waveguide model. In case of the inherently low-loss optical perturbations, the inverse designed pattern is optimized such that scattering at the output facet is decreased, which results in a reduction of the total scattering loss compared to the bare MMI. This is especially remarkable, because in contrast to the here shown 3D simulations, inverse design is based on a 2D effective index approximation, which does not include out-of-plane scattering.

## J. Estimation of fabrication alignment tolerances

One advantage of large-scale perturbations compared to perturbation sizes $\ll \lambda$ is that they are more resistant to fabrication tolerances. The simulated tolerance of the shallow etched device, that is shown in figure S10, against perturbation size is illustrated in figure S11a), where errors of up to $\pm 100$ nm result in less than 0.2 dB additional loss in the optimised output port. Another factor to consider is alignment accuracy of different mask layers during the fabrication process. For the experimental device presented in this work, the alignment problem is bypassed via the use of a single etch process, that is to say, the perturbation etch depth is the same as that of the rib structure. However, typical alignment overlay

Table S2. 3D simulations to estimate out-of-plane scattering – waveguide. Ratio of energy flux of scattering into the top and bottom planes in a 500 nm wide and 10 µm long waveguide with a single 750 nm long perturbation, covering the full waveguide width. The "shallow" etch depth is 120 nm.

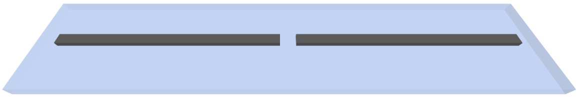

| out-of-plane scattering | bare | shallow etch | deep etch | optical pert. |
|---|---|---|---|---|
| top | 0.0% | 0.6% | 9.0% | 0.0% |
| bottom | 0.0% | 5.6% | 19.8% | 0.1% |

Table S3. 3D simulations to estimate out-of-plane scattering – optimized $1 \times 2$ MMI. Ratio of energy flux of scattering into the top and bottom planes in a $1 \times 2$ MMI with perturbation of $750 \times 750\,\text{nm}^2$ area. The "shallow" etch depth is 120 nm. The tested patterns are the same as shown in figure S10.

pattern "etched"

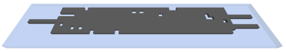

pattern "optical"

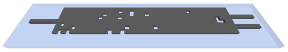

| out-of-plane scattering | bare | shallow etch | optical pert. |
|---|---|---|---|
| top | 0.1% | 0.5% | 0.2% |
| bottom | 1.1% | 2.9% | 0.9% |

accuracy of 20 nm for DUV lithography results in $< 0.1$ dB additional loss in this device, as demonstrated in figure S11b), thereby demonstrating the robustness of the technique.

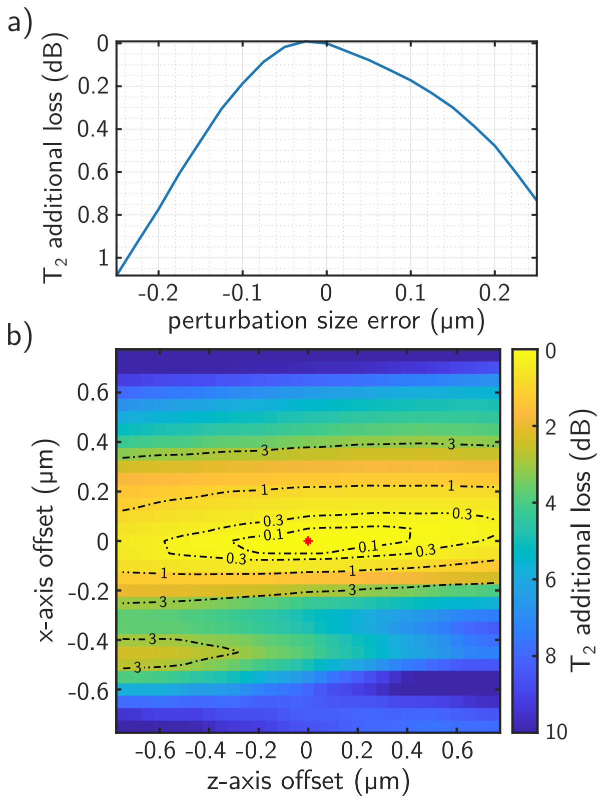


Figure S11. Simulated additional loss of optimised output port (T2) against (a) perturbation size error and (b) $x$- and $z$-axis offset for the pattern of the experimental shallow etched device (shown in Figure S10). 0 µm size error corresponds to $750 \times 750\,\text{nm}^2$ perturbations and the red star in (b) indicates the zero-offset position.
